# Supplementary material for: From Classification to Generation: Insights into Crosslingual Retrieval Augmented ICL
Source: arXiv:2311.06595 source file (2023-12-02)
Supplement: Supplementary file 1 [file appendix.tex]

Table~\ref{tab:8_templates_bloomz3b_task1} and Table~\ref{tab:6_templates_mbert_task1} show the F1-score results with different prompt templates in bloomz-3b model and mbert model.

\begin{table*}[]
\footnotesize
\centering \begin{tabular}{|lcccccc}
\toprule
\multicolumn{1}{c}{}          
& \multicolumn{3}{c}{k=1}    
& \multicolumn{3}{c}{k=3}   
\\ 
\multicolumn{1}{c}{bloomz-3b}     
& \multicolumn{1}{c}{precision} 
& \multicolumn{1}{c}{recall} 
& \multicolumn{1}{c}{f1-score}
& \multicolumn{1}{c}{precision} 
& \multicolumn{1}{c}{recall} & 
\multicolumn{1}{c}{f1-score} 
\\ \midrule
% \multicolumn{1}{c}{Negative}  
% & \multicolumn{1}{c}{0.58}     
% & \multicolumn{1}{c}{0.84}  
% & \multicolumn{1}{c}{0.69}    
% & \multicolumn{1}{c}{0.59}   
% & \multicolumn{1}{c}{0.88} 
% & \multicolumn{1}{c}{0.70} 
% \\ 
% \multicolumn{1}{c}{Neutral}  
% & \multicolumn{1}{c}{0.09}   
% & \multicolumn{1}{c}{0.00}   
% & \multicolumn{1}{c}{0.00}  
% & \multicolumn{1}{c}{0.08}  
% & \multicolumn{1}{c}{0.00}  
% & \multicolumn{1}{c}{0.00}  
% \\ 
% \multicolumn{1}{c}{Positive}  
% & \multicolumn{1}{c}{0.55}   
% & \multicolumn{1}{c}{0.49}   
% & \multicolumn{1}{c}{0.52}  
% & \multicolumn{1}{c}{0.58}  
% & \multicolumn{1}{c}{0.47}  
% & \multicolumn{1}{c}{0.52} 
% \\
\multicolumn{1}{c}{accuracy} 
& \multicolumn{1}{c}{}      
& \multicolumn{1}{c}{}    
& \multicolumn{1}{c}{0.57}   
& \multicolumn{1}{c}{}      
& \multicolumn{1}{c}{}      
& \multicolumn{1}{c}{0.58} 
\\ 
\multicolumn{1}{c}{macro avg}  
& \multicolumn{1}{c}{0.41}    
& \multicolumn{1}{c}{0.44}   
& \multicolumn{1}{c}{0.40}   
& \multicolumn{1}{c}{0.42}  
& \multicolumn{1}{c}{0.45}  
& \multicolumn{1}{c}{0.41} 
\\ 
\multicolumn{1}{c}{weighted avg} 
& \multicolumn{1}{c}{0.48}      
& \multicolumn{1}{c}{0.57} 
& \multicolumn{1}{c}{0.51}  
& \multicolumn{1}{c}{0.49}  
& \multicolumn{1}{c}{0.58}   
& \multicolumn{1}{c}{0.51}  
\\ \midrule
\multicolumn{1}{c}{mbert}     
& \multicolumn{1}{c}{precision} 
& \multicolumn{1}{c}{recall} 
& \multicolumn{1}{c}{f1-score}
& \multicolumn{1}{c}{precision} 
& \multicolumn{1}{c}{recall} & 
\multicolumn{1}{c}{f1-score} 
\\ \midrule
% \multicolumn{1}{c}{negative}  
% & \multicolumn{1}{c}{0.48}  
% & \multicolumn{1}{c}{0.24}  
% & \multicolumn{1}{c}{0.32}  
% & \multicolumn{1}{c}{0.48}   
% & \multicolumn{1}{c}{0.33}   
% & \multicolumn{1}{c}{0.39}
% \\ 
% \multicolumn{1}{c}{neutral}   
% & \multicolumn{1}{c}{0.21}   
% & \multicolumn{1}{c}{0.34}   
% & \multicolumn{1}{c}{0.26}  
% & \multicolumn{1}{c}{0.21} 
% & \multicolumn{1}{c}{0.28}  
% & \multicolumn{1}{c}{0.24}
% \\ 
% \multicolumn{1}{c}{positive}   
% & \multicolumn{1}{c}{0.27}    
% & \multicolumn{1}{c}{0.37}  
% & \multicolumn{1}{c}{0.31}  
% & \multicolumn{1}{c}{0.25}   
% & \multicolumn{1}{c}{0.33}   
% & \multicolumn{1}{c}{0.28}
% \\ 
\multicolumn{1}{c}{accuracy}
& \multicolumn{1}{c}{}       
& \multicolumn{1}{c}{}     
& \multicolumn{1}{c}{0.30} 
& \multicolumn{1}{c}{}      
& \multicolumn{1}{c}{}      
& \multicolumn{1}{c}{0.32}
\\ 
\multicolumn{1}{c}{macro avg}  
& \multicolumn{1}{c}{0.32}     
& \multicolumn{1}{c}{0.32}  
& \multicolumn{1}{c}{0.30}  
& \multicolumn{1}{c}{0.31}  
& \multicolumn{1}{c}{0.31}  
& \multicolumn{1}{c}{0.31}
\\ 
\multicolumn{1}{c}{weighted avg} 
& \multicolumn{1}{c}{0.36}    
& \multicolumn{1}{c}{0.30} 
& \multicolumn{1}{c}{0.30}  
& \multicolumn{1}{c}{0.36}  
& \multicolumn{1}{c}{0.32}  
& \multicolumn{1}{c}{0.33} 
\\ \bottomrule
\end{tabular}
\caption{Results of SentNoB test set using Hindi retrieval prompts}
\label{tab:results of SentNoB test bloomz-3b and mbert using hindi retrieval dataset}
\end{table*}

\begin{table*}[]
\footnotesize
\centering 
\begin{tabular}{lccc}
\hline
                                                        & zero-shot                                            & k=1                                            & k=3                                           \\ \hline
\multicolumn{4}{l}{\{text\} Direct Aggression, Indirect Aggression, or No Aggression?}                                                                                                                          \\
accuracy                                                & 0.53                                                 & 0.54                                           & 0.54                                          \\
macro avg                                               & 0.17                                                 & 0.18                                           & 0.18                                          \\
weighted avg                                            & 0.38                                                 & 0.38                                           & 0.38                                          \\ \hline
\multicolumn{4}{l}{\begin{tabular}[c]{@{}l@{}}Evaluate the text: '\{text\}'. Would you categorize it as absence of aggression, mild aggression, \\ or strong aggression?\end{tabular}}                          \\
accuracy                                                & 0.18                                                 & 0.23                                           & 0.23                                          \\
macro avg                                               & 0.17                                                 & 0.15                                           & 0.15                                          \\
weighted avg                                            & 0.13                                                 & 0.16                                           & 0.16                                          \\ \hline
\multicolumn{4}{l}{\begin{tabular}[c]{@{}l@{}}In the context of '\{text\}', which category best captures its aggression level: absence of aggression, \\ mild aggression, or strong aggression?\end{tabular}}   \\ 
accuracy                                                & 0.12                                                 & 0.15                                           & 0.16                                          \\
macro avg                                               & 0.1                                                  & 0.15                                           & 0.16                                          \\
weighted avg                                            & 0.06                                                 & 0.11                                           & 0.12                                          \\ \hline
\multicolumn{4}{l}{\begin{tabular}[c]{@{}l@{}}For the text: '\{text\}', ascertain its aggression scale: absence of aggression, mild aggression, or \\ strong aggression?\end{tabular}}                          \\
accuracy                                                & 0.19                                                 & 0.21                                           & 0.21                                          \\
macro avg                                               & 0.13                                                 & 0.14                                           & 0.14                                          \\
weighted avg                                            & 0.14                                                 & 0.16                                           & 0.15                                          \\ \hline
\multicolumn{4}{l}{\begin{tabular}[c]{@{}l@{}}From the following choices, which resonates with the theme of '\{text\}'? Options: No Intensity, \\ Low Intensity, High Intensity\end{tabular}}                   \\
accuracy                                                & 0.13                                                 & 0.24                                           & 0.19                                          \\
macro avg                                               & 0.1                                                  & 0.17                                           & 0.15                                          \\
weighted avg                                            & 0.12                                                 & 0.26                                           & 0.2                                           \\ \hline
\multicolumn{4}{l}{\begin{tabular}[c]{@{}l@{}}From the following choices, which resonates with the theme of '\{text\}'? Options: no intensity, \\ low intensity, high intensity\end{tabular}}                   \\
accuracy                                                & 0.23                                                 & 0.28                                           & 0.27                                          \\
macro avg                                               & 0.18                                                 & 0.22                                           & 0.2                                           \\
weighted avg                                            & 0.22                                                 & 0.31                                           & 0.26                                          \\ \hline
\multicolumn{4}{l}{\begin{tabular}[c]{@{}l@{}}In the context of the text '\{text\}', which of the following best describes its tone? Options: No \\ Intensity, Low Intensity, High Intensity\end{tabular}}      \\
accuracy                                                & 0.14                                                 & 0.2                                            & 0.15                                          \\
macro avg                                               & 0.11                                                 & 0.15                                           & 0.12                                          \\
weighted avg                                            & 0.1                                                  & 0.18                                           & 0.13                                          \\ \hline
\multicolumn{4}{l}{\begin{tabular}[c]{@{}l@{}}Reflecting on the statement '\{text\}', which aggressive level does it resonate with: non-aggressive, \\ slightly aggressive, or highly aggressive?\end{tabular}} \\
accuracy                                                & 0.33                                                 & 0.35                                           & 0.36                                          \\
macro avg                                               & 0.2                                                  & 0.2                                            & 0.17                                          \\
weighted avg                                            & 0.19                                                 & 0.2                                            & 0.24                                          \\ \hline
\end{tabular}
\caption{F1-score results with 8 prompt templates of Vio-Lens test using bloomz-3b model}
\label{tab:8_templates_bloomz3b_task1}
\end{table*}

\begin{table*}[]
\centering 
\begin{tabular}{lrrr}
\hline
             & \multicolumn{1}{l}{zero-shot} & \multicolumn{1}{l}{k=1} & \multicolumn{1}{l}{k=3} \\ \hline
\multicolumn{4}{l}{The text displays {[}MASK{]} aggression: \{text\}}                            \\
\multicolumn{4}{l}{verbalizer: direct, indirect, none}                                           \\ 
accuracy     & 0.36                          & 0.35                    & 0.36                    \\
macro avg    & 0.22                          & 0.23                    & 0.23                    \\
weighted avg & 0.31                          & 0.31                    & 0.31                    \\ \hline
\multicolumn{4}{l}{Considering aggressive tendencies, this is {[}MASK{]}: \{text\}}              \\
\multicolumn{4}{l}{verbalizer: overt, covert, absent}                                            \\ 
accuracy     & 0.1                           & 0.2                     & 0.17                    \\
macro avg    & 0.07                          & 0.17                    & 0.14                    \\
weighted avg & 0.03                          & 0.19                    & 0.15                    \\ \hline
\multicolumn{4}{l}{{[}From an aggression perspective, the text is {[}MASK{]}: \{text\}}          \\
\multicolumn{4}{l}{verbalizer: overt, covert, absent}                                            \\ 
accuracy     & 0.12                          & 0.22                    & 0.2                     \\
macro avg    & 0.09                          & 0.18                    & 0.16                    \\
weighted avg & 0.06                          & 0.21                    & 0.18                    \\ \hline
\multicolumn{4}{l}{The described behavior in \{text\} is {[}MASK{]} aggression.}                 \\
\multicolumn{4}{l}{verbalizer: explicit, implicit, neutral}                                      \\
accuracy     & 0.24                          & 0.36                    & 0.35                    \\
macro avg    & 0.19                          & 0.24                    & 0.23                    \\
weighted avg & 0.23                          & 0.31                    & 0.3                     \\ \hline
\multicolumn{4}{l}{The underlying theme in \{text\} is {[}MASK{]} aggression.}                   \\
\multicolumn{4}{l}{verbalizer: assaultive, indirect, peaceful}                                   \\ 
accuracy     & 0.22                          & 0.32                    & 0.33                    \\
macro avg    & 0.18                          & 0.21                    & 0.21                    \\
weighted avg & 0.21                          & 0.28                    & 0.29                    \\ \hline
\multicolumn{4}{l}{\{text\} is interpreted as {[}MASK{]} aggression.}                            \\
\multicolumn{4}{l}{verbalizer: assaultive, indirect, peaceful}                                   \\ 
accuracy     & 0.51                          & 0.49                    & 0.51                    \\
macro avg    & 0.23                          & 0.27                    & 0.25                    \\
weighted avg & 0.37                          & 0.37                    & 0.37                    \\ \hline
\end{tabular}
\caption{F1-score results with 6 prompt templates of Vio-Lens test using mBert model}
\label{tab:6_templates_mbert_task1}
\end{table*}
